# Supplementary material for: Conformal Language Modeling
Source: arXiv:2306.10193 source file (2024-06-01)
Supplement: Supplementary file 1 [file CNNDM_0.tex]

\begin{table}[h]
\caption{Example prediction sets for example from CNN/DM dataset, at $\alpha=0.3$, $\epsilon=0.7$}
\centering

\begin{tabular}{|p{0.12\linewidth} | p{0.6\linewidth} | p{0.12\linewidth} | p{0.08\linewidth}| }
\hline
& \textbf{Text} & \textbf{Score} & \textbf{Label} \\
\hline
Ref & A new poll has asked Brits and Americans questions about the royal baby.
Both nationalities favour a girl and want her to be a good role model.
UK's top names are Charlotte and Alice, while US likes Diana and Elizabeth. &  &  \\ \hline
Sample 1 & William and Kate are preparing for the birth of the second royal baby . \textbf{The survey reveals Brits and Americans want a baby girl .} Americans favour distinctively prominent royal names like Diana . James, Richard and Arthur are the most popular boys names . & 2.36e-01 & False \\\hline
Sample 2 & William and Kate are preparing for the birth of the second royal baby . \textbf{The survey reveals that both Brits and Americans want a baby girl .} Americans prefer distinctively prominent royal names such as Diana . In the UK, Charlotte is the leading name for a girl . James, Richard and Arthur are the most popular boys names . & 2.65e-01 & False \\\hline
Sample 3 & The survey reveals that Brits and Americans are on similar footing when it comes to the choice of a royal baby . Americans prefer distinctively prominent royal names, such as Diana or Elizabeth . Both Brits and Americans agree on James, Richard and Arthur as their favourite boys names . & 1.73e-01 & False \\\hline
Sample 4 & The survey reveals that Brits and Americans share similar views on names . Americans prefer distinctively prominent royal names, like Diana . In the UK, Charlotte is the leading name for a potential girl . While Brits favour Diana, Elizabeth and Victoria . & 7.89e-02 & True \\\hline
Sample 6 & The UK and US have been swept by royal baby fascination since 2013 . Both Brits and Americans have a preference for a baby girl . Survey reveals a landslide of 87\% of Americans and 7\% of Brits . Americans prefer distinctively prominent royal names like Diana . James, Richard and Arthur are the top three names for boys in both countries . & 1.97e-01 & False \\\hline
Sample 8 & William and Kate are currently prepping for the birth of the second royal baby . This has spurred guesses on the sex and name of the second child . Survey reveals Brits and Americans favour Charlotte, Alice and Alexandra . Americans prefer distinctively prominent royal names, Diana and Elizabeth . James, Richard and Arthur are the most popular boys names in the UK . & 1.34e-01 & False \\\hline
Sample 9 & William and Kate are preparing for the birth of the second royal baby . The survey reveals that Brits and Americans share similar views on name choices . Americans prefer distinctively prominent royal names like Diana, Elizabeth and Victoria . Both Brits and Americans agree on James, Richard and Arthur as top three boys names . & 7.82e-02 & False \\\hline
Sample 10 & William and Kate are currently expecting the second royal baby . \textbf{The survey reveals that both Brits and Americans want a baby girl .} Americans prefer distinctively prominent royal names like Diana . In the UK, Charlotte is the leading name for a girl . While Americans favour Diana, Elizabeth and Victoria . & 2.19e-01 & False \\\hline
Sample 11 & The UK and US have been swept by royal baby excitement . Both Brits and Americans want a baby girl, with Charlotte a leading name . Americans favour distinctively prominent royal names, Diana and Elizabeth . James, Richard and Arthur are the most popular boys names for the UK . & 1.04e-01 & False \\\hline
Sample 12 & The UK and US both want to see the second royal baby a girl . Survey reveals Americans prefer distinctively prominent royal names . Brits favour Charlotte, Alice and Alexandra as the top girls names . Americans favour Diana, Elizabeth and Victoria as the top three names . James, Richard and Arthur are the most popular boys names for the UK . & 2.27e-01 & False \\\hline
\end{tabular}
\label{tab:CNNDM_0}
\end{table}
