# Supplementary material for: Conformal Language Modeling
Source: arXiv:2306.10193 source file (2024-06-01)
Supplement: Supplementary file 2 [file CNNDM_5.tex]

\begin{table}[h]
\caption{Example prediction sets for example from CNN/DM dataset, at $\alpha=0.3$, $\epsilon=0.7$}
\centering

\begin{tabular}{|p{0.12\linewidth} | p{0.6\linewidth} | p{0.12\linewidth} | p{0.08\linewidth}| }
\hline
& \textbf{Text} & \textbf{Score} & \textbf{Label} \\
\hline
Ref & Aston Villa drew 3-3 with QPR in their Premier League clash on Monday.
Belgium striker Christian Benteke scored a hat-trick for the Villans.
Robert Green was embarrassed by a nutmeg from a cheeky ball boy. &  &  \\ \hline
Sample 1 & \textbf{QPR drew 3-3 with Aston Villa in Premier League on Monday night .} Christian Benteke scored a hat-trick to move three points clear of relegation . Ball boy decided to play a prank on the QPR goalkeeper as the clock was ticking . & 3.13e-01 & True \\\hline
Sample 2 & QPR drew 3-3 with Aston Villa in the Premier League on Monday night . Christian Benteke scored a hat-trick to move three points clear of relegation . Rangers host Chelsea at Loftus Park on Sunday in a bid to beat the drop . & 2.08e-01 & False \\\hline
Sample 4 & \textbf{QPR drew 3-3 with Aston Villa in Premier League on Monday night .} Ball boy who slipped over before retrieving the ball then rolled it between Green's legs . QPR goalkeeper Rob Green smiled as he struggled to retrieve the ball . The cheeky lad went on to roll the ball between the 35-year-old's legs . & 4.01e-01 & True \\\hline
Sample 5 & \textbf{QPR drew 3-3 with Aston Villa in Premier League on Monday night .} \textbf{Rangers goalkeeper Rob Green was embarrassed by ball boy .} Youngster rolled the ball between Green's legs . & 3.09e-01 & True \\\hline
Sample 6 & \textbf{QPR drew 3-3 with Aston Villa in Premier League on Monday night .} Christian Benteke scored a hat-trick to move three points clear of relegation . Ball boy decided to prank QPR goalkeeper Rob Green with a nutmeg . & 1.64e-01 & True \\\hline
Sample 7 & \textbf{QPR drew 3-3 with Aston Villa in Premier League on Monday night .} \textbf{Rangers goalkeeper Rob Green was played a prank by a ball boy .} Youngster roll the ball between Green's legs as he attempts to retrieve it . & 1.44e-01 & True \\\hline
\end{tabular}
\label{tab:CNNDM_5}
\end{table}
