# Supplementary material for: Conformal Language Modeling
Source: arXiv:2306.10193 source file (2024-06-01)
Supplement: Supplementary file 3 [file CNNDM_6.tex]

\begin{table}[h]
\caption{Example prediction sets for example from CNN/DM dataset, at $\alpha=0.3$, $\epsilon=0.7$}
\centering

\begin{tabular}{|p{0.12\linewidth} | p{0.6\linewidth} | p{0.12\linewidth} | p{0.08\linewidth}| }
\hline
& \textbf{Text} & \textbf{Score} & \textbf{Label} \\
\hline
Ref & Pauline Bruce's neighbour Yvonne plagued her for seven years.
Yvonne made silent phone calls day and night and shouted abuse.
Taunted her husband, Tony, when he was diagnosed with terminal cancer.
'I was frightened for our lives,' said Pauline, from Ludlow, Shropshire. &  &  \\ \hline
Sample 1 & \textbf{Pauline Bruce was terrorised by her neighbour Yvonne Ireland Evans .} She went from being a friend, to a nuisance, and then a threat . Yvonne attacked Pauline's son John with secateurs . She also taunted her dying husband Tony and his family . Pauline says she was terrified for her and her family's lives . & 1.90e-01 & False \\\hline
Sample 2 & Pauline Bruce was terrorised by Yvonne Ireland Evans for seven years . She went from being a friend, to a nuisance, and then a threat to her family . Yvonne attacked Pauline's son with secateurs, and threatened to kill him . Couple were finally rescued after Yvonne rang 999 and stayed with them . & 2.43e-01 & False \\\hline
Sample 3 & \textbf{Pauline Bruce was terrorised by her neighbour Yvonne Ireland Evans .} She went from being a friend, to a nuisance, and then a threat . Yvonne attacked her son with secateurs, and taunted her husband . She didn't even show compassion when Tony died of terminal cancer . & 3.06e-01 & False \\\hline
Sample 4 & \textbf{Pauline Bruce was terrorised by her neighbour Yvonne Ireland Evans .} She went from being a friend, to a nuisance, and then a threat . Yvonne attacked Pauline's son John with secateurs . She didn't care when Tony died of terminal cancer . Finally diagnosed with dementia, she was jailed for 14 years . & 1.62e-01 & False \\\hline
Sample 5 & Pauline Bruce was terrorised by Yvonne Ireland Evans for seven years . She went from being a friend, to a nuisance, and then a threat to her family . Yvonne attacked Pauline's son John with secateurs . She also taunted her dying husband Tony and his family . & 2.47e-01 & False \\\hline
\end{tabular}
\label{tab:CNNDM_6}
\end{table}
