# Supplementary material for: Conformal Language Modeling
Source: arXiv:2306.10193 source file (2024-06-01)
Supplement: Supplementary file 4 [file CNNDM_8.tex]

\begin{table}[h]
\caption{Example prediction sets for example from CNN/DM dataset, at $\alpha=0.3$, $\epsilon=0.7$}
\centering

\begin{tabular}{|p{0.12\linewidth} | p{0.6\linewidth} | p{0.12\linewidth} | p{0.08\linewidth}| }
\hline
& \textbf{Text} & \textbf{Score} & \textbf{Label} \\
\hline
Ref & Heated open-air swimming pool to open on the Thames in two years' time.
Celebrity backers Tracy Emin and David Walliams speeded the plans along.
The social enterprise scheme is set to benefit local groups and the elderly.
Pools will use sophisticated filtration system to clean polluted river water. &  &  \\ \hline
Sample 1 & \textbf{Thames Bath Lido will sit near Blackfriars Bridge and open in two years .} \textbf{Original idea was conceived by three Londoners who dreamt of bringing the beautiful lakes of Zurich to the capital .} The Lido will incorporate two pools, a 25 meter lap pool and a training pool . Artist Tracy Emin has said she could not believe how underused the Thames is . \textbf{David Walliams has said he will be the first to jump in if the water is clean enough .} & 6.57e-01 & False \\\hline
Sample 2 & \textbf{Thames Bath Lido will sit near Blackfriars Bridge and open in two years .} \textbf{Original idea was conceived by three Londoners who dreamt of bringing the beautiful lakes of Zurich to the capital .} The Lido will incorporate two pools, a 25 meter lap pool and a training pool . Artist Tracy Emin and David Walliams have also pledged their support . & 6.59e-01 & False \\\hline
\end{tabular}
\label{tab:CNNDM_8}
\end{table}
