# Supplementary material for: Conformal Language Modeling
Source: arXiv:2306.10193 source file (2024-06-01)
Supplement: Supplementary file 5 [file CNNDM_9.tex]

\begin{table}[h]
\caption{Example prediction sets for example from CNN/DM dataset, at $\alpha=0.3$, $\epsilon=0.7$}
\centering

\begin{tabular}{|p{0.12\linewidth} | p{0.6\linewidth} | p{0.12\linewidth} | p{0.08\linewidth}| }
\hline
& \textbf{Text} & \textbf{Score} & \textbf{Label} \\
\hline
Ref & WARNING: GRAPHIC CONTENT.
Footage was released along with other key pieces of evidence.
Video played in court shows truck pulling up to driveway of burger stand.
His pickup then backs up after a struggle and runs over Sloan's leg.
The vehicle is then seen plowing over Carter, killing him.
Other pieces of evidence included an hour-long interview with Cle 'Bone' Sloan, who survived being run over by the Death Row Records co-founder.
A number of images taken immediately after his arrest were also released.
Close-ups of his face were intended to show injuries he sustained after being punched by Sloan. &  &  \\ \hline
Sample 1 & Cle 'Bone' Sloan told police Suge Knight growled 'I'll kill you' in January . He claims rap mogul then yanked on gear stick and 'everything went black' Sloan claims they had a 'disaster' after Knight threatened to kill him . Knight, co-founder of Death Row Records, denies killing Terry Carter . He was also accused of ramming over Sloan in his pick-up truck . \textbf{Images of Knight have been released along with key pieces of evidence .} & 1.41e-01 & False \\\hline
Sample 2 & Cle 'Bone' Sloan told officers Suge Knight growled 'I'll kill you' in car . He claims rap mogul then yanked on gear stick and 'everything went black' Sloan claims they had a 'match of a lifetime' when Knight killed Terry Carter . Knight, co-founder of Death Row Records, is on trial for Carter's murder . He is also accused of ramming over Sloan's head with his truck . Earlier this week, a picture of Knight with virtually no facial injuries was released . & 6.64e-02 & False \\\hline
Sample 4 & Cle 'Bone' Sloan told officers Suge Knight growled 'I'll kill you' in car . He claims it happened before Knight rammed him over in Compton parking lot . Sloan also claims Knight appeared to be reaching for a gun on the passenger seat . Images of Knight show he had virtually no facial injuries when arrested . Knight, co-founder of Death Row Records, denies killing Terry Carter . & 1.01e-01 & False \\\hline
Sample 5 & Cle 'Bone' Sloan told officers Suge Knight growled 'I'll kill you' in new video . Clip was released along with key pieces of evidence as trial began . Knight, co-founder of Death Row Records, is on trial for killing Terry Carter and trying to kill Cle 'Bone' Sloan in a parking lot in Compton on January 18 . He claims he saw Knight reaching for a gun on the passenger seat . Sloan says: 'After that, everything turned into a dream' & 1.58e-01 & False \\\hline
Sample 6 & Cle 'Bone' Sloan told officers Suge Knight growled 'I'll kill you' in car . He claims that was moment before Knight allegedly drove over him with his truck . Sloan claims Knight reached for a gun on passenger seat and yanked on gear stick . Knight, co-founder of Death Row Records, denies killing Terry Carter . He also allegedly tried to kill Sloan by running him over in his pick-up truck . Images of Knight show him with virtually no facial injuries when arrested . Close-ups taken by detectives show he had only slight black eye . & 8.17e-02 & False \\\hline
Sample 8 & Cle 'Bone' Sloan told police Suge Knight growled 'I'll kill you' in January . He claims Knight then yanked on the gear stick and 'everything went black' Sloan claims the pair exchanged blows in a parking lot in Compton . Knight, co-founder of Death Row Records, has denied the killing . He is accused of killing Terry Carter and trying to kill Cle 'Bone' Sloan . Photos of Knight show he had virtually no facial injuries when arrested . Close-ups taken by detectives show he only had a slight black eye . & 1.20e-01 & False \\\hline
Sample 9 & Cle 'Bone' Sloan told police Suge Knight growled 'I'll kill you' in January . He claims rap mogul then yanked on gear stick and 'everything went black' Sloan claims they had a 'fight' and Knight threatened to kill him in his car . Knight, co-founder of Death Row records, is on trial for murder . He is accused of killing Terry Carter and running over Cle 'Bone' Sloan . Sloan says he believes he was 'choked on the gear stick' and struck him . & 3.19e-01 & False \\\hline
Sample 10 & Cle 'Bone' Sloan told police Suge Knight growled 'I'll kill you' in January . He claims rap mogul then yanked on gear stick and 'everything went black' Sloan claims they had a 'match of a lifetime' when they met at the scene . Knight, co-founder of Death Row Records, is on trial for Terry Carter murder . He is also accused of ramming over Sloan with his pick-up truck . & 2.10e-01 & False \\\hline
\end{tabular}
\label{tab:CNNDM_9}
\end{table}
