# Supplementary material for: Conformal Language Modeling
Source: arXiv:2306.10193 source file (2024-06-01)
Supplement: Supplementary file 6 [file CNNDM_7.tex]

\begin{table}[h]
\caption{Example prediction sets for example from CNN/DM dataset, at $\alpha=0.3$, $\epsilon=0.7$}
\centering

\begin{tabular}{|p{0.12\linewidth} | p{0.6\linewidth} | p{0.12\linewidth} | p{0.08\linewidth}| }
\hline
& \textbf{Text} & \textbf{Score} & \textbf{Label} \\
\hline
Ref & Boris Johnson to move centre stage in Tory election campaign next week.
London Mayor to make a high profile joint appearance with David Cameron.
Comes amid surprise he was not at the Tory manifesto launch this week. &  &  \\ \hline
Sample 1 & Boris Johnson will make high-profile joint appearance with David Cameron . He has been largely invisible at national level despite being second best known Tory . Calls from Conservative MPs for Mr Johnson to be 'weaponised' in election . & 2.74e-01 & False \\\hline
Sample 3 & Boris Johnson will make high-profile joint appearance with David Cameron . UK's second best known Tory will be 'weaponised' in election campaign . Lord Bell says Tories' campaign is 'dreadful, risk averse, boring' & 4.09e-01 & True \\\hline
Sample 10 & \textbf{Boris Johnson will move centre stage in Tory election campaign next week .} He will make high-profile joint appearance with David Cameron, sources say . Calls from Conservative MPs for Mr Johnson to be 'weaponised' in election . & 3.35e-01 & False \\\hline
\end{tabular}
\label{tab:CNNDM_7}
\end{table}
